# Supplementary material for: Single-image coherent reconstruction of objects and humans
Source: arXiv:2408.08086 source file (2024-08-15)
Supplement: Supplementary file 1 [file X_suppl.tex]

\clearpage
\setcounter{page}{1}
\maketitlesupplementary

% Optional math commands from https://github.com/goodfeli/dlbook_notation.

\section{Implementation Details}

The Human-Human Interaction loss - $L_{HHI-Loss}$ is optimized using ADAM with learning rate $2e-3$ for 100 iterations. The trainable parameters are translation $t^{i} \in \mathbb{R}^3$ and intrinsic scale $s^{i} \in \mathbb{R}$  for the $i^{th}$ human. We initialized the optimization with the human poses estimated using Sec 3.1(in the paper).

ADAM optimizer is used to optimize occlusion-aware silhouette loss with a learning rate of $2e-3$ for 200 iterations and edge maps $E(M)$ are computed using $MaxPool(M)$ - $M$ with a filter size of 7.

We optimize the joint loss - $L_{joint-loss}$  using ADAM with a learning rate $3e-4$ for 500 iterations. The trainable parameters are translation $t^{i} \in \mathbb{R}^3$ and intrinsic scale $s^{i} \in \mathbb{R}$  for the $i^{th}$ human and, rotation $R^{j} \in SO(3)$, translation $t^{j} \in \mathbb{R}^3$ and $s^{j} \in \mathbb{R}$ for the $j^{th}$ object instance jointly. The loss weights $\lambda_{i}$ are tuned qualitatively on the COCO-2017 val set.We initialized the optimization with the human poses estimated in Sec 3.2 (in the paper) and the best object pose estimated in Sec.3.3 (in the paper) per object instance.

\section{Evaluation Equations}
We compare our method with PHOSA, ROMP, and BEV by reconstructing the scenes and comparing the degree of mesh collisions for human-human $E_{H-col}$ and human-object $E_{HO-col}$ and incorrect depth ordering for human-human $E_{H-depth}$ and human-object $E_{HO-depth}$ interactions that results from each method. We randomly sample the total $T$ number of images from the COCO2017 test set and for each image, reconstruction is performed via all methods to calculate $E_{H-col}$, $E_{HO-col}$, $E_{H-depth}$ and $E_{HO-depth}$. Finally, we determine the average value for all these for the different methods. A lower score implies better reconstruction. The equations used to calculate these are as follows, which indicate the average value of mesh collision loss among human-human reconstructions and humans-object reconstructions:
\begin{gather}
    E_{HO-col} = \frac{1}{T} * \sum_{k=1}^{T} \Bigl(\sum_{j=1}^{N_{o}^{k}}  \Bigl (\sum_{i=1}^{N_{h}^{k}} L_{h_{i}o_{j}}^{k} + L_{o_{j}h_{i}}^{k} \Bigl) \Bigl) 
\end{gather}
where, $L_{h_{i}o_{j}}^{k}$ and $L_{o_{j}h_{i}}^{k}$ are defined in the manuscript under Human-Object collision loss Sec 3.4 (in the paper).

where, $L_{ij}^{k}$ is defined in the manuscript under human-human collision loss Sec 3.2(in the paper)

\begin{gather}
    E_{H-col} = \frac{1}{T} * \sum_{k=1}^{T} \Bigl(\sum_{j=1}^{N^{k}}  \Bigl (\sum_{i=1 i\neq j}^{N^{k}} L_{ij}^{k} \Bigl) \Bigl) 
\end{gather}

The other evaluation parameters indicate the average value of depth disparity for human-human and human-object reconstruction across all photos.

\begin{multiline}
        E_{HO-depth} = \frac{1}{T} * \sum_{k=1}^{T} \Bigl(\sum_{p \in S_{h}U S_{o}} \log(1 + \exp(D_{y(p)}^{k}(p) - D_{\Bar{y}(p)}^{k}(p) )) \Bigl)
\end{multiline}

\begin{multiline}
       E_{H-depth}= \frac{1}{T} * \sum_{k=1}^{T} \Bigl(\sum_{p \in S_{h}} \log(1 + \exp(D_{y(p)}^{k}(p) - D_{\Bar{y}(p)}^{k}(p) )) \Bigl) 
\end{multiline}

\section{Bounding Box Overlap Criteria} \label{sec:c}
Given two objects $i$ and $j$, we first determine a tight bounding box around these objects. Let us call them $box_{i}$ and $box_{j}$ respectively. One important thing to note here is that boxes are axis-aligned. Let's say that the corners of $box_i$ are $l_i = (x_1, y_1, z_1)$
and $r_i = (X_1, Y_1, Z_1)$ where $X_1>x_1$, $Y_1>y_1$ and $Z_1>z_1$. Similarly, we can represent corners of $box_j$ as $l_j = (x_2, y_2, z_2)$
and $r_j = (X_2, Y_2, Z_2)$ where $X_2>x_2$, $Y_2>y_2$ and $Z_2>z_2$. The way to check for an overlap is to compare the intervals $[x_1, X_1]$
and $[x_2, X_2]$, and if they don't overlap, there's no intersection. Do the same for the y intervals, and the z intervals. 

\begin{lstlisting}[language=Python]
def CheckOverlap(l_i,r_i,l_j,r_j):
    x_1, y_1, z_1 = l_i
    X_1, Y_1, Z_1 = r_i
    x_2, y_2, z_2 = l_j
    X_2, Y_2, Z_2 = r_j
    if x_1 > X_2 or x_2 > X_1:
        return false
    if y_1 > Y_2 or y_2 > Y_1:
        return false
    if z_1 > Z_2 or z_2 > Z_1:
        return false
    return true
\end{lstlisting}

% we remove those objects which have iou greater than 0.3
\section{IOU Thresholding} \label{sec:d}

 In this paper, one of our contributions is a novel approach aimed at enhancing the segmentation mask of occluded objects. Our methodology leverages image in-painting for object removal, incorporating an Intersection over Union (IOU) threshold set at $> 0.3$. It is worth noting that this threshold is flexible, allowing for experimentation with various values. Our choice of this threshold is rooted in empirical observations, where we noted that objects with an IOU exceeding 0.3 resulted in noticeable enhancements in reconstruction quality. Conversely, when the IOU was below 0.3, the reconstruction results obtained by PHOSA closely resembled those produced by using our method. To illustrate this distinction, we provide several examples showcasing reconstruction cases where the IOU falls below and exceeds the 0.3 threshold.

\begin{figure}[h] 
\includegraphics[scale = 0.35]{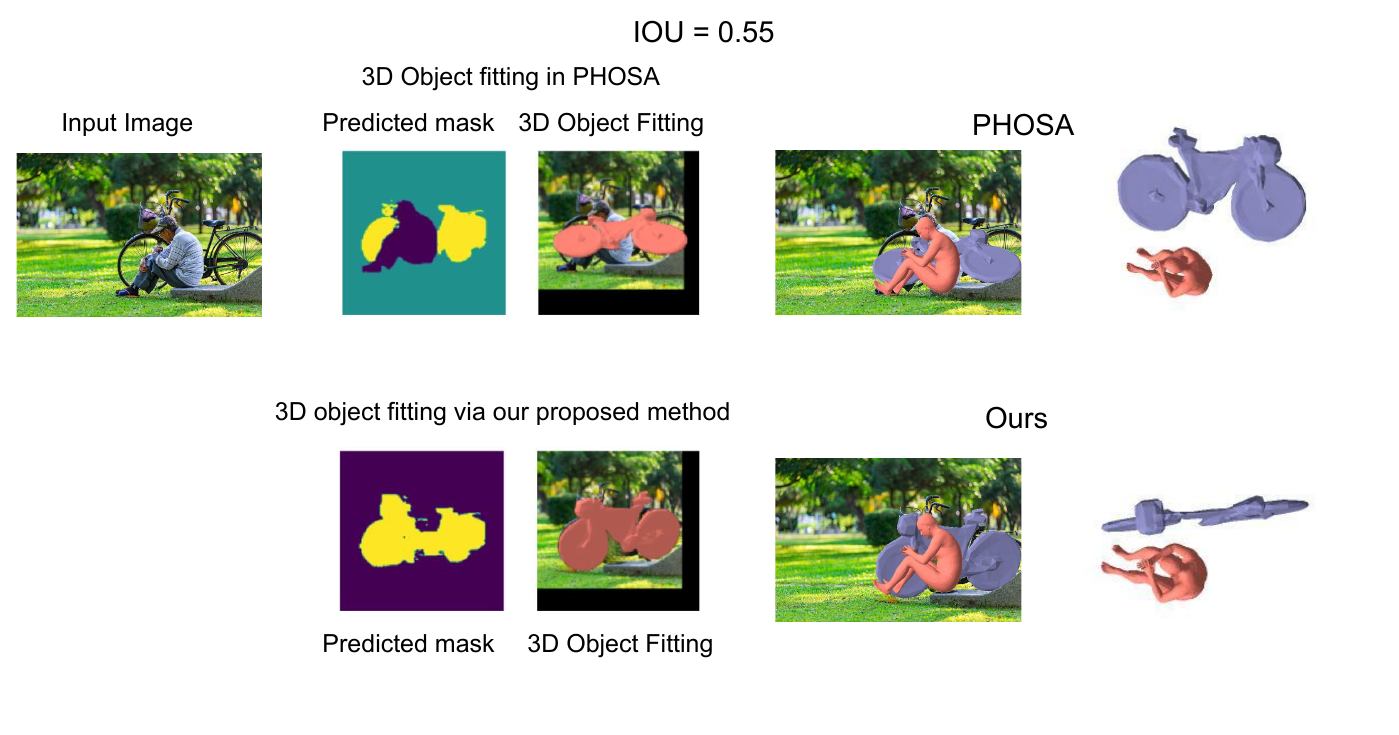}
\centering
\end{figure}

\vspace{1.5cm}

\begin{figure}[h] 
\includegraphics[scale = 0.35, page =2]{images/iclr-iou-results-new.pdf}
\centering
\end{figure}

\begin{figure}[h] 
\includegraphics[scale = 0.35, page =3]{images/iclr-iou-results-new.pdf}
\centering
\end{figure}

\vspace{1.5cm}

\begin{figure}[h] 
\includegraphics[scale = 0.35, page =4]{images/iclr-iou-results-new.pdf}
\centering
\end{figure}

\begin{figure}[h] 
\includegraphics[scale = 0.35, page=5]{images/iclr-iou-results-new.pdf}
\centering
\end{figure}

\vspace{1.5cm}

\begin{figure}[h] 
\includegraphics[scale = 0.35, page =6]{images/iclr-iou-results-new.pdf}
\centering
\end{figure}

\begin{figure}[h] 
\includegraphics[scale = 0.35, page =7]{images/iclr-iou-results-new.pdf}
\centering
\end{figure}

\vspace{1.5cm}

\begin{figure}[h] 
\includegraphics[scale = 0.35, page =8]{images/iclr-iou-results-new.pdf}
\centering
\end{figure}

\begin{figure}[h] 
\includegraphics[scale = 0.35]{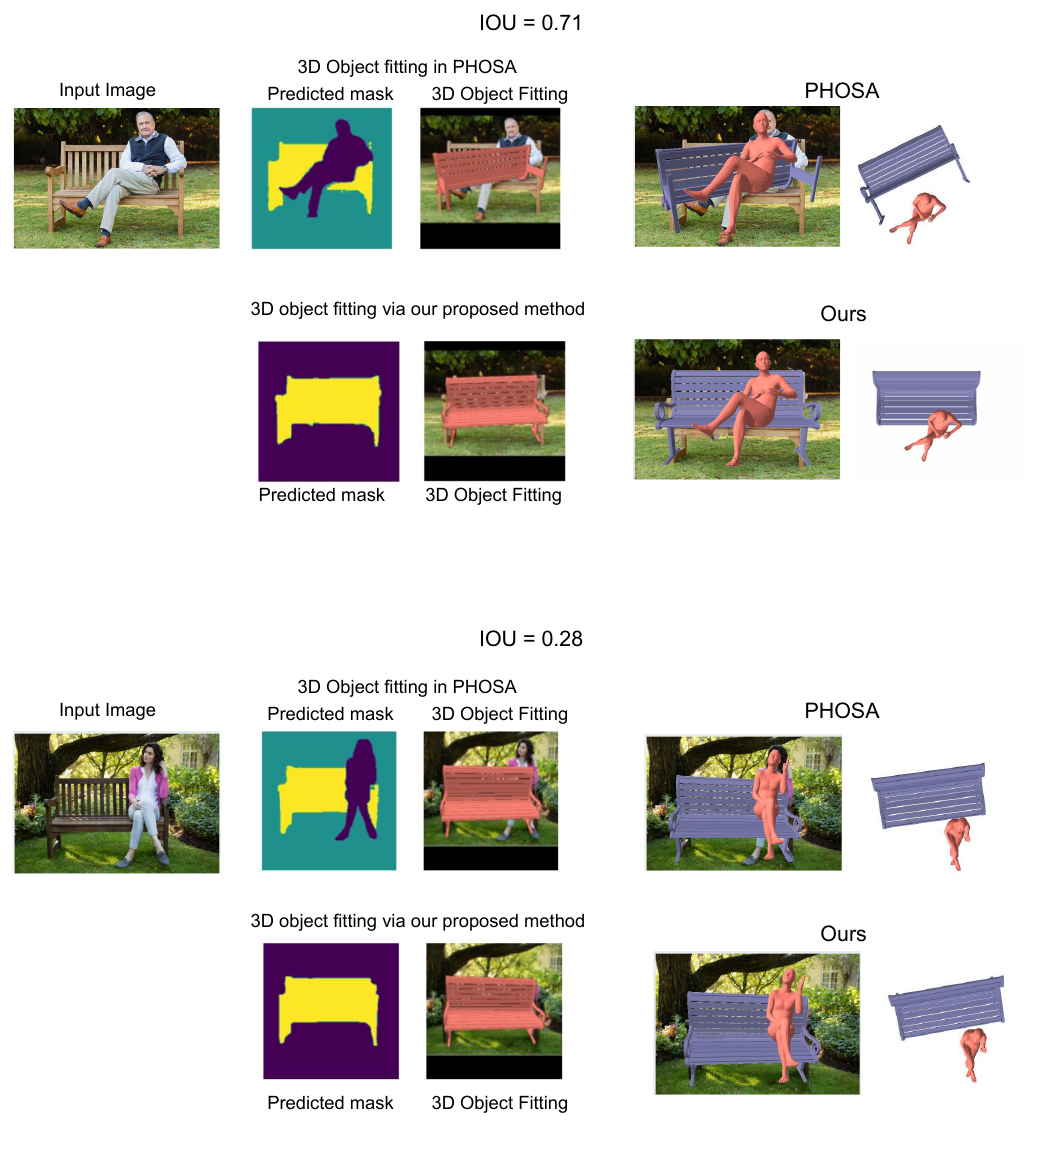}
\centering
\end{figure}
